# Supplementary material for: Methodology to Construct Large Realizations of Perfectly Hyperuniform Disordered Packings
Source: arXiv:1901.10006 ancillary file (2019-06-01)
Supplement: Supplementary file 1 [file SupplementaryMaterials.pdf]

# Supplemental Materials: Methodology to Construct Large Realizations of Perfectly Hyperuniform Disordered Packings

Jaeuk Kim[1] and Salvatore Torquato[1,2,3,4,*]
[1] Department of Physics, Princeton University, Princeton, New Jersey 08544, USA
[2] Department of Chemistry, Princeton University, Princeton, New Jersey 08544, USA
[3] Princeton Institute for the Science and Technology of Materials, Princeton University, Princeton, New Jersey 08544, USA
[4] Program in Applied and Computational Mathematics, Princeton University, Princeton, New Jersey 08544, USA

## I. HYPERUNIFORM PACKINGS DERIVED FROM VORONOI TESSELLATIONS

Here, we provide additional simulation data that are not presented in Sec. V in the main text.

### A. Progenitor packings for Voronoi tessellations

Here, we summarize the simulation parameters employed to generate progenitor packings that are used to obtain Voronoi tessellations.

TABLE S1. The number of progenitor packings used in the tessellation-based procedure. Packings are defined by initial packing fraction $\phi_{\text{init}}$ and particle number $N$. For saturated RSA packings with $\phi_{\text{init}} = \phi_{\text{sat}}$, the number of particles can vary for each realization. For reference, the saturated packing fractions of RSA packings are $\phi_{\text{sat}} = 0.5470735(28)$ and $0.3841307(21)$ in $d = 2$ and 3, respectively [1]. Here, HSL stands for equilibrium hard-sphere liquids below the freezing point.

| Models | $\phi_{\text{init}}$ | $N$ | | | | |
|---|---|---|---|---|---|---|
| | | $10^3$ | $10^4$ | $10^5$ | $10^6$ | $10^7$ |
| 2D RSA | $\phi_{\text{sat}}$<br>0.41025<br>0.27350<br>0.13675 | $10^4$ | $10^3$ | $10^2$ | 50 | 25 |
| 3D RSA | $\phi_{\text{sat}}$<br>0.288<br>0.192<br>0.096 | $10^4$ | $10^3$ | $10^2$ | 50 | - |
| 2D HSL | 0.65<br>0.40<br>0.20 | $10^4$ | $10^3$ | $10^2$ | - | - |
| 3D HSL | 0.45<br>0.30<br>0.20 | $10^4$ | $10^3$ | $10^2$ | 50 | - |

To exactly generate saturated RSA packing, we employed the voxel-list algorithm, developed by Zhang and Torquato [1]. The number of sampled configurations are listed in Table. S1.

TABLE S2. The number of lattice packings with spatially uncorrelated vacancies, used in the tessellation-based procedure. Packings are defined by the vacancy concentration $c$ and the initial particle number $N_s$. Thus, particle number is $N = (1-c)N_s$.

| Models | $N_s$ | $c$ | | |
|---|---|---|---|---|
| | | 0.1 | 0.2 | 0.4 |
| $\mathbb{Z}^2$ lattice with vacancies | $10^6$ | | 100 | |
| | $25 \times 10^6$ | | 50 | |
| | $100 \times 10^6$ | | 20 | |
| $\mathbb{Z}^3$ lattice with vacancies | $10^6$ | | 100 | |
| | $27 \times 10^6$ | | 50 | |

Equilibrium hard-sphere liquids in $\mathbb{R}^2$ and $\mathbb{R}^3$ are simulated via the Monte Carlo method in canonical ensemble. Beginning with the initial triangular (FCC) lattice arrangements in $d = 2$ (3), we randomly remove some particles to have $N$ particles. Subsequently, we adjust the maximal distance of trial moves satisfying that its average acceptance ratio for 10 MC cycles becomes $0.3 \pm 0.005$, where 1 MC cycle implies $N$ trial moves (i.e., 1 trial move per particle). Then, we keep the system evolving until it is equilibrated in such a manner that the relative standard deviation in the contact value of the radial distribution function $g_2(r = D^+)$ for 4 successive MC cycles becomes less than $10^{-3}$. After equilibration, we sample a configuration every 10000 MC cycles. The number of sampled configurations is listed in Table. S1. Using the same analysis in Ref. [84] in the main text, we obtain theoretical prediction of $\tilde{\chi}_V(0)$ for 3D equilibrium hard-sphere liquids with the packing fraction $\phi_{\text{init}}$ as follows:

$$\tilde{\chi}_V(0) = \frac{\phi^2(1-\phi_{\text{init}})^4}{\rho(1+4\phi_{\text{init}}+4{\phi_{\text{init}}}^2-4{\phi_{\text{init}}}^3+{\phi_{\text{init}}}^4)}. \tag{S1}$$

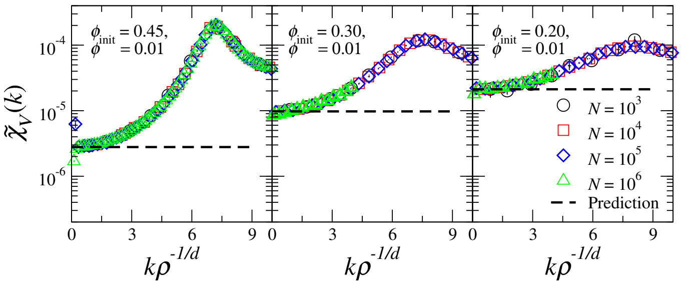


FIG. S1. Simulation results for the spectral densities $\tilde{\chi}_V(k)$ of 3D equilibrium hard-sphere liquids with various values of packing fraction $\phi_{\text{init}}$ and sample size $N$. "Prediction" represents $\tilde{\chi}_V(0)$, obtained by Eq. (S1).

A lattice packing with uncorrelated vacancies are generated by randomly removing $cN_s$ particles from an initial perfect $\mathbb{Z}^d$-lattice packing of $N_s$ particles.

## B. Maximal packing fractions

TABLE. S3, S4, and S5 summarize maximal packing fractions of constructed sphere packings derived from Voronoi tessellations.

While there is a tendency that the maximal packing fraction slowly decreases as system size grows, we can straightforwardly show that it is bounded below for saturated RSA packings. For saturated RSA packings in $\mathbb{R}^d$ ($d > 1$), their maximal packing fractions is estimated as follows:

$$\phi^{(2)}_{\text{max}} \equiv \min\left\{\frac{v_1(R)}{|C_j|}\right\} = \frac{v_1(R)}{\max\{|C_j|\}} \tag{S2}$$

$$> \frac{v_1(R)}{2^d\, v_1(R)} = \frac{1}{2^d}, \tag{S3}$$

where $R$ is the particle radius in a progenitor packing. In Eq. (S3), we use the fact that any Voronoi cell of a saturated RSA packing should be fully covered by a sphere of volume $2^d\, v_1(R)$, i.e., $|C_j| < 2^d\, v_1(R)$ for $j = 1, \cdots, N$. Here, we note that $\phi^{(2)}_{\text{max}} \le \phi^{(1)}_{\text{max}} \le \phi_{\text{max}}$.

TABLE S3. Maximal packing fractions of the packings constructed from the progenitor RSA packings of packing fraction $\phi_{\text{init}}$. The maximal packing fractions $\phi^{(2)}_{\text{max}}$ and $\phi^{(1)}_{\text{max}}$ are defined by Eq. (19) and Fig. 4 in the main text. Here, values in the square brackets represent the minimal values that we observed.

| $d$ | $\phi_{\text{init}}$ | $N$ | $\phi^{(1)}_{\text{max}}$ | | $\phi^{(2)}_{\text{max}}$ | | $d$ | $\phi_{\text{init}}$ | $N$ | $\phi^{(1)}_{\text{max}}$ | | $\phi^{(2)}_{\text{max}}$ | |
|---|---|---|---|---|---|---|---|---|---|---|---|---|---|
| | | $10^7$ | 0.360(4) | [0.3473] | 0.305(4) | [0.2999] | | | $10^7$ | - | [-] | - | [-] |
| | | $10^6$ | 0.366(4) | [0.3573] | 0.314(5) | [0.2993] | | | $10^6$ | 0.252(7) | [0.2374] | 0.231(5) | [0.2203] |
| | $\phi_{\text{sat}}$ | $10^5$ | 0.380(7) | [0.3578] | 0.325(7) | [0.3070] | | $\phi_{\text{sat}}$ | $10^5$ | 0.264(6) | [0.2477] | 0.240(6) | [0.2220] |
| | | $10^4$ | 0.395(10) | [0.3581] | 0.341(10) | [0.3050] | | | $10^4$ | 0.277(7) | [0.2436] | 0.253(7) | [0.2071] |
| | | $10^3$ | 0.418(14) | [0.3626] | 0.362(13) | [0.3086] | | | $10^3$ | 0.294(10) | [0.2395] | 0.269(10) | [0.2083] |
| | | $10^7$ | 0.217(12) | [0.1792] | 0.1769(5) | [0.1650] | | | $10^7$ | - | [-] | - | [-] |
| | | $10^6$ | 0.234(8) | [0.2156] | 0.188(5) | [0.1768] | | | $10^6$ | 0.183(4) | [0.1760] | 0.158(3) | [0.1522] |
| | 0.41025 | $10^5$ | 0.252(10) | [0.2189] | 0.201(8) | [0.1792] | | 0.2880 | $10^5$ | 0.1920(6) | [0.1795] | 0.1662(4) | [0.1544] |
| | | $10^4$ | 0.274(13) | [0.2193] | 0.217(10) | [0.1796] | | | $10^4$ | 0.205(7) | [0.1680] | 0.177(6) | [0.1554] |
| 2D | | $10^3$ | 0.301(17) | [0.2218] | 0.239(13) | [0.1704] | 3D | | $10^3$ | 0.220(9) | [0.1742] | 0.190(8) | [0.1514] |
| | | $10^7$ | 0.106(5) | [0.0921] | 0.076(5) | [0.0655] | | | $10^7$ | - | [-] | - | [-] |
| | | $10^6$ | 0.116(6) | [0.0909] | 0.084(4) | [0.0707] | | | $10^6$ | 0.103(4) | [0.0926] | 0.083(3) | [0.0732] |
| | 0.2735 | $10^5$ | 0.132(8) | [0.1017] | 0.094(5) | [0.0793] | | 0.192 | $10^5$ | 0.1111(5) | [0.0973] | 0.0892(4) | [0.0793] |
| | | $10^4$ | 0.150(11) | [0.1034] | 0.106(7) | [0.0803] | | | $10^4$ | 0.1230(2) | [0.0936] | 0.0976(2) | [0.0795] |
| | | $10^3$ | 0.176(16) | [0.1030] | 0.1232(10) | [0.0739] | | | $10^3$ | 0.1376(1) | [0.0998] | 0.1083(1) | [0.0766] |
| | | $10^7$ | 0.044(2) | [0.0395] | 0.028(1) | [0.0249] | | | $10^7$ | - | [-] | - | [-] |
| | | $10^6$ | 0.049(4) | [0.0395] | 0.030(2) | [0.0231] | | | $10^6$ | 0.043(3) | [0.0336] | 0.030(2) | [0.0256] |
| | 0.13675 | $10^5$ | 0.056(5) | [0.0438] | 0.035(2) | [0.0285] | | 0.096 | $10^5$ | 0.0479(3) | [0.0399] | 0.0337(2) | [0.0282] |
| | | $10^4$ | 0.067(7) | [0.0435] | 0.040(3) | [0.0292] | | | $10^4$ | 0.0547(1) | [0.0400] | 0.0374(1) | [0.0273] |
| | | $10^3$ | 0.083(10) | [0.0409] | 0.048(5) | [0.0275] | | | $10^3$ | 0.0647(1) | [0.0394] | 0.0433(1) | [0.0267] |

TABLE S4. Maximal packing fractions of the constructed sphere packings according to the progenitor packings from equilibrium hard-sphere liquids. The maximal packing fractions $\phi^{(2)}_{\text{max}}$ and $\phi^{(1)}_{\text{max}}$ are defined by Eq. (19) and Fig. 4 in the main text. Here, values in the square brackets represent the minimal values that we observed.

| $d$ | $\phi_{\text{init}}$ | $N$ | $\phi^{(1)}_{\text{max}}$ | | $\phi^{(2)}_{\text{max}}$ | | $d$ | $\phi_{\text{init}}$ | $N$ | $\phi^{(1)}_{\text{max}}$ | | $\phi^{(2)}_{\text{max}}$ | |
|---|---|---|---|---|---|---|---|---|---|---|---|---|---|
| | | $10^6$ | - | | - | | | | $10^6$ | 0.307(8) | [0.2799] | 0.287(7) | [0.2682] |
| | 0.65 | $10^5$ | 0.437(1) | [0.4067] | 0.400(1) | [0.3611] | | 0.45 | $10^5$ | 0.3226(9) | [0.2909] | 0.3002(9) | [0.2709] |
| | | $10^4$ | 0.470(1) | [0.3741] | 0.428(1) | [0.3360] | | | $10^4$ | 0.3599(4) | [0.3064] | 0.3375(4) | [0.2948] |
| | | $10^3$ | 0.5053(2) | [0.3842] | 0.4632(2) | [0.3661] | | | $10^3$ | 0.3603(1) | [0.2998] | 0.3378(1) | [0.2793] |
| | | $10^6$ | - | | - | | | | $10^6$ | 0.169(4) | [0.1550] | 0.146(5) | [0.1356] |
| 2D | 0.4 | $10^5$ | 0.200(1) | [0.1733] | 0.1567(8) | [0.1308] | 3D | 0.3 | $10^5$ | 0.1813(7) | [0.1576] | 0.1554(7) | [0.1253] |
| | | $10^4$ | 0.2259(4) | [0.1828] | 0.1772(3) | [0.1378] | | | $10^4$ | 0.1961(3) | [0.1553] | 0.1700(2) | [0.1311] |
| | | $10^3$ | 0.2585(2) | [0.1721] | 0.2026(2) | [0.1294] | | | $10^3$ | 0.217(12) | [0.1605] | 0.187(10) | [0.1392] |
| | | $10^6$ | - | | - | | | | $10^6$ | 0.098(4) | [0.0855] | 0.079(4) | [0.0691] |
| | 0.2 | $10^5$ | 0.0833(7) | [0.0649] | 0.0551(3) | [0.0453] | | 0.2 | $10^5$ | 0.1069(5) | [0.0890] | 0.0860(4) | [0.0656] |
| | | $10^4$ | 0.0979(3) | [0.0640] | 0.0639(2) | [0.0478] | | | $10^4$ | 0.1189(2) | [0.0909] | 0.0945(2) | [0.0733] |
| | | $10^3$ | 0.1188(1) | [0.0608] | 0.0762(1) | [0.0446] | | | $10^3$ | 0.1354(96) | [0.0920] | 0.1070(72) | [0.0647] |

### C. Values of extrapolated $\tilde{\chi}_V(0)$

The limit values of $\lim_{k\to 0}\tilde{\chi}_V(k)$ for the constructed sphere packings are estimated by computing the spectral density $\tilde{\chi}_V(k_{\text{min}})$ at the smallest wavenumber and by extrapolating simulation results with a non-linear curve $y=\tilde{\chi}_V(0)+a_1x^4$. In the non-linear regression, we take errors in $\tilde{\chi}_V(k)$ into account. Then, for RSA packings, equilibrium hard-sphere liquids, and their constructed sphere packings, values of hyperuniform metric $H$ are computed as follows:

$$H=\begin{cases}\dfrac{\tilde{\chi}_V(k_{\text{min}})}{\tilde{\chi}_V(peak)}, & \text{Progenitor packings}\\ \dfrac{\tilde{\chi}_V(0)}{\tilde{\chi}_V(peak)}, & \text{Constructed packings,}\end{cases} \tag{S4}$$

where $\tilde{\chi}_V(peak)$ represents the spectral density at the first dominant non-Bragg peak. Tables S6, S7, and S8 summarize simulation data.

TABLE S5. Maximal packing fractions of the constructed sphere packings from imperfect $\mathbb{Z}^d$ packings with uncorrelated point vacancy concentration $c$. The maximal packing fractions $\phi^{(2)}_{\max}$ and $\phi^{(1)}_{\max}$ are defined by Eq. (19) and Fig. 4 in the main text. Here, values in the square brackets represent the minimal values that we observed.

| $d$ | $c$ | $N_s$ | $\phi^{(1)}_{\max}$ | | $\phi^{(2)}_{\max}$ | | $d$ | $c$ | $N_s$ | $\phi^{(1)}_{\max}$ | | $\phi^{(2)}_{\max}$ | |
|---|---|---|---|---|---|---|---|---|---|---|---|---|---|
| 2D | 0.10 | $100 \times 10^6$ | 0.229(7) | [0.2142] | 0.213(8) | [0.1953] | 3D | 0.10 | - | - | | - | |
| | | $25 \times 10^6$ | 0.236(11) | [0.2081] | 0.223(12) | [0.1904] | | | $27 \times 10^6$ | 0.198(8) | [0.1792] | 0.1967(8) | [0.1792] |
| | | $1 \times 10^6$ | 0.267(11) | [0.2327] | 0.267(11) | [0.2327] | | | $1 \times 10^6$ | 0.221(9) | [0.1888] | 0.220(10) | [0.1871] |
| | 0.20 | $100 \times 10^6$ | 0.173(8) | [0.1611] | 0.159(7) | [0.1442] | | 0.20 | - | - | | - | |
| | | $25 \times 10^6$ | 0.183(8) | [0.1608] | 0.169(8) | [0.1511] | | | $27 \times 10^6$ | 0.151(6) | [0.1392] | 0.147(6) | [0.1239] |
| | | $1 \times 10^6$ | 0.208(11) | [0.1687] | 0.191(11) | [0.1514] | | | $1 \times 10^6$ | 0.169(8) | [0.1456] | 0.165(10) | [0.1233] |
| | 0.40 | $100 \times 10^6$ | 0.113(6) | [0.1014] | 0.097(6) | [0.0812] | | 0.40 | - | - | | - | |
| | | $25 \times 10^6$ | 0.118(6) | [0.1062] | 0.103(5) | [0.0920] | | | $27 \times 10^6$ | 0.099(4) | [0.0906] | 0.089(4) | [0.0774] |
| | | $1 \times 10^6$ | 0.137(8) | [0.1148] | 0.119(7) | [0.0991] | | | $1 \times 10^6$ | 0.110(6) | [0.0931] | 0.103(6) | [0.0769] |

TABLE S6. Values of hyperuniform metric $H$ for RSA packings ($d = 2, 3$) and corresponding constructed packings. Spectral density $\tilde{\chi}_V(k_{\min})$ at the minimum wavenumber and the extrapolated values of $\tilde{\chi}_V(0)$ are summarized.

| $d$ | $\phi_{\text{init}}$ | $N$ | Progenitor packing | | Constructed packing | | |
|---|---|---|---|---|---|---|---|
| | | | $\tilde{\chi}_V(k_{\min})$ | $H$ | $\tilde{\chi}_V(k_{\min})$ | $\tilde{\chi}_V(0)$ | $H$ |
| 2D | $\phi_{\text{sat}}$ | $10^7$ | $5.93(49) \times 10^{-6}$ | $3.5(3) \times 10^{-2}$ | $6.14(54) \times 10^{-18}$ | $2.29(54) \times 10^{-18}$ | $1.36(32) \times 10^{-14}$ |
| | | $10^6$ | $6.05(43) \times 10^{-6}$ | $3.6(3) \times 10^{-2}$ | $4.56(36) \times 10^{-16}$ | $5.38(359) \times 10^{-17}$ | $3.20(214) \times 10^{-13}$ |
| | | $10^5$ | $5.13(25) \times 10^{-6}$ | $3.0(2) \times 10^{-2}$ | $4.54(29) \times 10^{-14}$ | $6.07(292) \times 10^{-15}$ | $3.80(183) \times 10^{-11}$ |
| | | $10^4$ | $5.96(13) \times 10^{-6}$ | $3.5(1) \times 10^{-2}$ | $1.94(4) \times 10^{-12}$ | $4.05(441) \times 10^{-14}$ | $2.53(276) \times 10^{-10}$ |
| | | $10^3$ | $5.84(3) \times 10^{-6}$ | $3.51(8) \times 10^{-2}$ | $4.74(3) \times 10^{-10}$ | $1.37(3) \times 10^{-10}$ | $8.57(20) \times 10^{-7}$ |
| | 0.41025 | $10^7$ | $1.08(10) \times 10^{-5}$ | $8.0(7) \times 10^{-2}$ | $1.34(15) \times 10^{-17}$ | $4.67(146) \times 10^{-18}$ | $3.36(105) \times 10^{-14}$ |
| | | $10^6$ | $1.01(7) \times 10^{-5}$ | $7.4(5) \times 10^{-2}$ | $1.15(11) \times 10^{-15}$ | $2.65(107) \times 10^{-16}$ | $1.90(77) \times 10^{-12}$ |
| | | $10^5$ | $9.59(46) \times 10^{-6}$ | $7.0(3) \times 10^{-2}$ | $1.03(6) \times 10^{-13}$ | $1.51(64) \times 10^{-14}$ | $1.16(49) \times 10^{-10}$ |
| | | $10^4$ | $9.49(15) \times 10^{-6}$ | $7.0(1) \times 10^{-2}$ | $1.04(2) \times 10^{-11}$ | $9.86(226) \times 10^{-13}$ | $7.53(173) \times 10^{-9}$ |
| | | $10^3$ | $9.69(5) \times 10^{-6}$ | $7.11(4) \times 10^{-2}$ | $1.06(1) \times 10^{-9}$ | $3.04(7) \times 10^{-10}$ | $2.33(5) \times 10^{-6}$ |
| | 0.2735 | $10^7$ | $2.19(19) \times 10^{-5}$ | $1.9(2) \times 10^{-1}$ | $4.99(60) \times 10^{-17}$ | $1.15(60) \times 10^{-17}$ | $1.01(52) \times 10^{-13}$ |
| | | $10^6$ | $2.37(17) \times 10^{-5}$ | $2.1(1) \times 10^{-1}$ | $5.00(54) \times 10^{-15}$ | $1.33(53) \times 10^{-15}$ | $1.17(47) \times 10^{-11}$ |
| | | $10^5$ | $2.33(12) \times 10^{-5}$ | $2.1(1) \times 10^{-1}$ | $4.68(29) \times 10^{-13}$ | $8.77(289) \times 10^{-14}$ | $7.70(253) \times 10^{-10}$ |
| | | $10^4$ | $2.42(4) \times 10^{-5}$ | $2.13(3) \times 10^{-1}$ | $4.66(9) \times 10^{-11}$ | $6.18(99) \times 10^{-12}$ | $5.42(87) \times 10^{-8}$ |
| | | $10^3$ | $2.45(1) \times 10^{-5}$ | $2.15(1) \times 10^{-1}$ | $4.64(3) \times 10^{-9}$ | $2.06(3) \times 10^{-9}$ | $1.81(3) \times 10^{-5}$ |
| | 0.13675 | $10^7$ | $5.12(43) \times 10^{-5}$ | $5.3(4) \times 10^{-1}$ | $1.54(18) \times 10^{-16}$ | $3.12(182) \times 10^{-17}$ | $2.95(172) \times 10^{-13}$ |
| | | $10^6$ | $5.32(38) \times 10^{-5}$ | $5.5(4) \times 10^{-1}$ | $1.44(12) \times 10^{-14}$ | $2.03(120) \times 10^{-15}$ | $1.92(114) \times 10^{-11}$ |
| | | $10^5$ | $4.94(24) \times 10^{-5}$ | $5.1(2) \times 10^{-1}$ | $1.45(9) \times 10^{-12}$ | $2.40(92) \times 10^{-13}$ | $2.27(87) \times 10^{-9}$ |
| | | $10^4$ | $5.35(8) \times 10^{-5}$ | $5.53(8) \times 10^{-1}$ | $1.48(3) \times 10^{-10}$ | $1.86(31) \times 10^{-11}$ | $1.76(30) \times 10^{-7}$ |
| | | $10^3$ | $5.36(3) \times 10^{-5}$ | $5.54(3) \times 10^{-1}$ | $1.48(1) \times 10^{-8}$ | $8.86(10) \times 10^{-9}$ | $8.38(10) \times 10^{-5}$ |
| 3D | $\phi_{\text{sat}}$ | $10^6$ | $5.69(22) \times 10^{-6}$ | $4.27(22) \times 10^{-2}$ | $6.44(32) \times 10^{-12}$ | $1.97(31) \times 10^{-12}$ | $1.51(24) \times 10^{-8}$ |
| | | $10^5$ | $5.57(16) \times 10^{-6}$ | $4.17(12) \times 10^{-2}$ | $1.39(5) \times 10^{-10}$ | $4.51(54) \times 10^{-11}$ | $3.45(41) \times 10^{-7}$ |
| | | $10^4$ | $5.66(5) \times 10^{-6}$ | $4.36(4) \times 10^{-2}$ | $2.91(3) \times 10^{-9}$ | $9.08(34) \times 10^{-10}$ | $7.15(27) \times 10^{-6}$ |
| | | $10^3$ | $5.76(2) \times 10^{-6}$ | $4.52(1) \times 10^{-2}$ | $6.03(2) \times 10^{-8}$ | $1.16(2) \times 10^{-8}$ | $9.14(19) \times 10^{-5}$ |
| | 0.288 | $10^6$ | $7.72(34) \times 10^{-6}$ | $6.93(30) \times 10^{-2}$ | $5.87(31) \times 10^{-12}$ | $1.39(31) \times 10^{-12}$ | $1.27(28) \times 10^{-8}$ |
| | | $10^5$ | $7.25(20) \times 10^{-6}$ | $6.50(24) \times 10^{-2}$ | $2.00(7) \times 10^{-10}$ | $4.66(76) \times 10^{-11}$ | $4.28(71) \times 10^{-7}$ |
| | | $10^4$ | $7.50(7) \times 10^{-6}$ | $6.68(6) \times 10^{-2}$ | $4.34(5) \times 10^{-9}$ | $1.35(5) \times 10^{-9}$ | $1.21(5) \times 10^{-5}$ |
| | | $10^3$ | $7.80(2) \times 10^{-6}$ | $7.13(2) \times 10^{-2}$ | $8.96(3) \times 10^{-8}$ | $1.63(4) \times 10^{-8}$ | $1.48(3) \times 10^{-4}$ |
| | 0.192 | $10^6$ | $1.62(7) \times 10^{-5}$ | $1.70(8) \times 10^{-1}$ | $1.61(9) \times 10^{-11}$ | $3.77(85) \times 10^{-12}$ | $3.90(88) \times 10^{-8}$ |
| | | $10^5$ | $1.62(4) \times 10^{-5}$ | $1.71(6) \times 10^{-1}$ | $5.80(21) \times 10^{-10}$ | $1.62(22) \times 10^{-10}$ | $1.67(23) \times 10^{-6}$ |
| | | $10^4$ | $1.65(2) \times 10^{-5}$ | $1.77(2) \times 10^{-1}$ | $1.243(15) \times 10^{-8}$ | $3.57(16) \times 10^{-9}$ | $3.77(17) \times 10^{-5}$ |
| | | $10^3$ | $1.700(5) \times 10^{-5}$ | $1.84(1) \times 10^{-1}$ | $2.515(9) \times 10^{-7}$ | $3.71(12) \times 10^{-8}$ | $3.97(13) \times 10^{-4}$ |
| | 0.096 | $10^6$ | $4.46(21) \times 10^{-5}$ | $5.49(25) \times 10^{-1}$ | $5.66(32) \times 10^{-11}$ | $1.44(32) \times 10^{-11}$ | $1.66(36) \times 10^{-7}$ |
| | | $10^5$ | $4.21(11) \times 10^{-5}$ | $5.18(19) \times 10^{-1}$ | $1.93(7) \times 10^{-9}$ | $4.96(71) \times 10^{-10}$ | $5.69(83) \times 10^{-6}$ |
| | | $10^4$ | $4.26(4) \times 10^{-5}$ | $5.40(6) \times 10^{-1}$ | $4.108(48) \times 10^{-8}$ | $1.09(5) \times 10^{-8}$ | $1.27(6) \times 10^{-4}$ |
| | | $10^3$ | $4.35(1) \times 10^{-5}$ | $5.52(2) \times 10^{-1}$ | $8.078(30) \times 10^{-7}$ | $2.03(4) \times 10^{-7}$ | $2.40(4) \times 10^{-3}$ |

TABLE S7. Values of hyperuniform metric $H$ for equilibrium hard-sphere liquids ($d = 2$ and 3) and corresponding constructed packings. Spectral density $\tilde{\chi}_V(k_{\min})$ at the minimum wavenumber and the extrapolated values of $\tilde{\chi}_V(0)$ are summarized.

| $d$ | $\phi_{\text{init}}$ | $N$ | Progenitor packing $\tilde{\chi}_V(k_{\min})$ | | Progenitor packing $H$ | | Constructed packing $\tilde{\chi}_V(k_{\min})$ | | Constructed packing $\tilde{\chi}_V(0)$ | | Constructed packing $H$ | |
|---|---|---|---|---|---|---|---|---|---|---|---|---|
| 2D | 0.65 | $10^5$ | 4.39(32) | $\times 10^{-6}$ | 1.26(10) | $\times 10^{-2}$ | 4.21(20) | $\times 10^{-14}$ | 2.03(32) | $\times 10^{-14}$ | 6.03(98) | $\times 10^{-11}$ |
| | | $10^4$ | 2.641(15) | $\times 10^{-6}$ | 8.07(6) | $\times 10^{-3}$ | 1.85(2) | $\times 10^{-10}$ | 4.71(19) | $\times 10^{-11}$ | 1.49(6) | $\times 10^{-7}$ |
| | | $10^3$ | 2.627(13) | $\times 10^{-6}$ | 7.95(4) | $\times 10^{-3}$ | 2.90(2) | $\times 10^{-10}$ | 5.63(19) | $\times 10^{-11}$ | 1.75(6) | $\times 10^{-7}$ |
| | 0.40 | $10^5$ | 1.640(78) | $\times 10^{-5}$ | 1.05(7) | $\times 10^{-1}$ | 2.89(19) | $\times 10^{-13}$ | 6.7(19) | $\times 10^{-14}$ | 4.45(130) | $\times 10^{-10}$ |
| | | $10^4$ | 1.477(23) | $\times 10^{-5}$ | 1.01(2) | $\times 10^{-1}$ | 2.66(5) | $\times 10^{-11}$ | 3.89(56) | $\times 10^{-12}$ | 2.75(40) | $\times 10^{-8}$ |
| | | $10^4$ | 1.493(7) | $\times 10^{-5}$ | 1.04(1) | $\times 10^{-1}$ | 2.63(2) | $\times 10^{-9}$ | 5.64(18) | $\times 10^{-10}$ | 4.07(13) | $\times 10^{-6}$ |
| | 0.20 | $10^5$ | 4.10(20) | $\times 10^{-5}$ | 3.80(18) | $\times 10^{-1}$ | 1.13(7) | $\times 10^{-12}$ | 2.48(76) | $\times 10^{-13}$ | 2.20(67) | $\times 10^{-9}$ |
| | | $10^4$ | 4.196(7) | $\times 10^{-5}$ | 3.89(9) | $\times 10^{-1}$ | 1.05(2) | $\times 10^{-10}$ | 1.34(22) | $\times 10^{-11}$ | 1.19(20) | $\times 10^{-7}$ |
| | | $10^3$ | 4.227(2) | $\times 10^{-5}$ | 3.97(3) | $\times 10^{-1}$ | 1.07(1) | $\times 10^{-8}$ | 3.10(7) | $\times 10^{-9}$ | 2.80(7) | $\times 10^{-5}$ |
| 3D | 0.45 | $10^6$ | 1.693(45) | $\times 10^{-6}$ | 8.52(23) | $\times 10^{-3}$ | 9.02(32) | $\times 10^{-12}$ | -1.36(318) | $\times 10^{-13}$ | 7(16) | $\times 10^{-10}$ |
| | | $10^5$ | 6.26(74) | $\times 10^{-6}$ | 3.07(37) | $\times 10^{-2}$ | 1.10(5) | $\times 10^{-10}$ | 3.92(54) | $\times 10^{-11}$ | 1.94(27) | $\times 10^{-7}$ |
| | | $10^4$ | 2.921(31) | $\times 10^{-6}$ | 1.52(2) | $\times 10^{-2}$ | 2.49(3) | $\times 10^{-8}$ | 5.90(39) | $\times 10^{-9}$ | 3.10(21) | $\times 10^{-5}$ |
| | | $10^3$ | 1.143(2) | $\times 10^{-5}$ | 6.27(1) | $\times 10^{-2}$ | 2.09(0) | $\times 10^{-7}$ | 1.35(2) | $\times 10^{-8}$ | 7.46(9) | $\times 10^{-5}$ |
| | 0.30 | $10^6$ | 8.55(35) | $\times 10^{-6}$ | 6.96(29) | $\times 10^{-2}$ | 8.91(47) | $\times 10^{-12}$ | 9.2(47) | $\times 10^{-13}$ | 7.6(39) | $\times 10^{-9}$ |
| | | $10^5$ | 9.56(26) | $\times 10^{-6}$ | 7.78(24) | $\times 10^{-2}$ | 3.59(13) | $\times 10^{-10}$ | 1.01(13) | $\times 10^{-10}$ | 8.4(11) | $\times 10^{-7}$ |
| | | $10^4$ | 9.871(88) | $\times 10^{-6}$ | 8.27(8) | $\times 10^{-2}$ | 7.74(9) | $\times 10^{-9}$ | 2.46(9) | $\times 10^{-9}$ | 2.08(8) | $\times 10^{-5}$ |
| | | $10^3$ | 1.036(3) | $\times 10^{-5}$ | 8.83(3) | $\times 10^{-2}$ | 1.57(1) | $\times 10^{-7}$ | 3.27(6) | $\times 10^{-8}$ | 2.80(6) | $\times 10^{-4}$ |
| | 0.20 | $10^6$ | 1.794(72) | $\times 10^{-5}$ | 1.84(7) | $\times 10^{-1}$ | 2.10(11) | $\times 10^{-11}$ | 7.7(32) | $\times 10^{-13}$ | 8.0(33) | $\times 10^{-9}$ |
| | | $10^5$ | 2.213(61) | $\times 10^{-5}$ | 2.27(7) | $\times 10^{-1}$ | 8.99(33) | $\times 10^{-10}$ | 4.96(53) | $\times 10^{-11}$ | 5.11(55) | $\times 10^{-7}$ |
| | | $10^4$ | 2.132(19) | $\times 10^{-5}$ | 2.19(2) | $\times 10^{-1}$ | 1.86(2) | $\times 10^{-8}$ | 4.28(15) | $\times 10^{-9}$ | 4.45(16) | $\times 10^{-5}$ |
| | | $10^3$ | 2.14(54) | $\times 10^{-5}$ | 2.22(56) | $\times 10^{-1}$ | 3.74(2) | $\times 10^{-7}$ | 6.36(17) | $\times 10^{-9}$ | 5.32(76) | $\times 10^{-5}$ |

TABLE S8. Values of spectral density $\tilde{\chi}_V(k_{\min})$ at the minimum wavenumber and the extrapolated values of $\tilde{\chi}_V(0)$ for the imperfect $\mathbb{Z}^d$-lattice packings and the constructed sphere packings.

| $d$ | $c$ | $N_s$ | $\tilde{\chi}_V(k_{\min})$ Progenitor | | $\tilde{\chi}_V(k_{\min})$ Constructed | | $\tilde{\chi}_V(0)$ Constructed | |
|---|---|---|---|---|---|---|---|---|
| 2D | 0.10 | $100 \times 10^6$ | 5.93(49) | $\times 10^{-6}$ | 6.14(54) | $\times 10^{-18}$ | 2.29(54) | $\times 10^{-18}$ |
| | | $25 \times 10^6$ | 6.05(43) | $\times 10^{-6}$ | 4.56(36) | $\times 10^{-16}$ | 5.4(36) | $\times 10^{-17}$ |
| | | $10^6$ | 5.13(26) | $\times 10^{-6}$ | 4.54(29) | $\times 10^{-14}$ | 6.1(29) | $\times 10^{-15}$ |
| | 0.20 | $100 \times 10^6$ | 1.08(10) | $\times 10^{-5}$ | 1.34(15) | $\times 10^{-17}$ | 4.7(15) | $\times 10^{-18}$ |
| | | $25 \times 10^6$ | 1.01(7) | $\times 10^{-5}$ | 1.15(11) | $\times 10^{-15}$ | 2.6(11) | $\times 10^{-16}$ |
| | | $10^6$ | 9.59(46) | $\times 10^{-6}$ | 1.03(6) | $\times 10^{-13}$ | 1.52(64) | $\times 10^{-14}$ |
| | 0.40 | $100 \times 10^6$ | 2.19(19) | $\times 10^{-5}$ | 4.99(60) | $\times 10^{-17}$ | 1.15(60) | $\times 10^{-17}$ |
| | | $25 \times 10^6$ | 2.37(17) | $\times 10^{-5}$ | 5.00(54) | $\times 10^{-15}$ | 1.33(53) | $\times 10^{-15}$ |
| | | $10^6$ | 2.33(11) | $\times 10^{-5}$ | 4.68(29) | $\times 10^{-13}$ | 8.8(29) | $\times 10^{-14}$ |
| 3D | 0.10 | $27 \times 10^6$ | 5.69(22) | $\times 10^{-6}$ | 6.44(32) | $\times 10^{-12}$ | 1.97(31) | $\times 10^{-12}$ |
| | | $10^6$ | 5.57(16) | $\times 10^{-6}$ | 1.39(5) | $\times 10^{-10}$ | 4.52(54) | $\times 10^{-11}$ |
| | 0.20 | $27 \times 10^6$ | 7.72(33) | $\times 10^{-6}$ | 5.87(3) | $\times 10^{-12}$ | 1.39(31) | $\times 10^{-12}$ |
| | | $10^6$ | 7.25(20) | $\times 10^{-6}$ | 2.00(7) | $\times 10^{-10}$ | 4.67(76) | $\times 10^{-11}$ |
| | 0.40 | $27 \times 10^6$ | 1.62(7) | $\times 10^{-5}$ | 1.61(9) | $\times 10^{-11}$ | 3.77(85) | $\times 10^{-12}$ |
| | | $10^6$ | 1.62(4) | $\times 10^{-5}$ | 5.80(21) | $\times 10^{-10}$ | 1.62(2) | $\times 10^{-10}$ |

## II. SPHERE TESSELLATIONS

Simulation parameters employed in this work are summarized in TABLE. S9.

TABLE S9. The prescribed cell number $N$ in every stage for our coated-disks models. The upper bound on cell volumes is denoted by $v_{\max}$, and $|\mathcal{V}_d|$ is volume of the simulation box. For each parameter, we obtain 50 and 20 configurations when $v_{\max}/|\mathcal{V}_d| = 10^{-3}$ and $10^{-4}$, respectively.

| Cell-volume scalings | | $v_{\max}/\lvert\mathcal{V}_d\rvert$ | |
|---|---|---|---|
| Type | Parameter | $10^{-3}$ | $10^{-4}$ |
| Power-law | 1.5 | 383 | - |
| | 1.6 | 438 | 4375 |
| | 1.7 | 487 | 4868 |
| | 1.8 | 532 | - |
| Exponential | 1.05 | 48 | - |
| | 1.10 | 91 | - |
| | 1.20 | 167 | - |

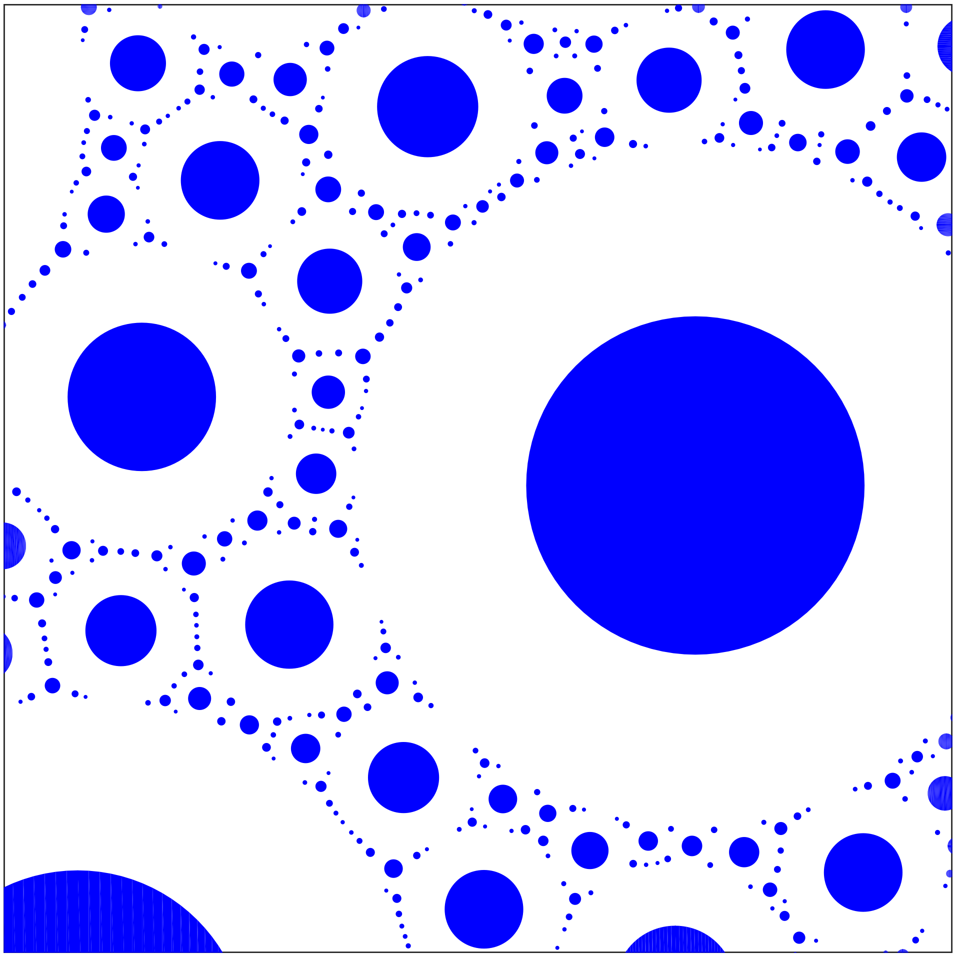

FIG. S2. An enlarged portion of Fig. 11 in the main text (×8 magnification). This packing is generated via a power-law scaling with $p = 1.5$ up to the 400th stage.

[1] G. Zhang and S. Torquato, "Precise algorithm to generate random sequential addition of hard hyperspheres at saturation," Phys. Rev. E **88**, 053312 (2013).
